# Supplementary material for: On Fair Ordering and Differential Privacy
Source: arXiv:2501.05535 source file (2025-01-09)
Supplement: Supplementary file 1 [file appendix.tex]

\section{Enjoy}
\subsection{Theorem 2 Proof}
Let $r,r'$ be two requests such that $r\sim r'$. By Assumption~\ref{assumption:bound_on_noise}, there exists a bound $\lambda$ such that $\lambda$ is the $\ell_1$-sensitivity of $score$. Since $\mathcal{A}$ is $\epsilon$-differentially private, for some fixed $s \in \mathcal{A}(score(r))$, we have
\begin{align*}
\text{Pr} [\mathcal{A}(score(r))=s] &\leq e^{\epsilon} \text{Pr}[\mathcal{A}(score(r'))=s] \\
\text{Pr} [\mathcal{A}(score(r'))=s] &\leq e^{\epsilon} \text{Pr}[\mathcal{A}(score(r))=s]
\end{align*}
\noindent Assume \[\text{Pr} [\mathcal{A}(score(r))=s] \leq \text{Pr}[\mathcal{A}(score(r'))=s]\]
We want to prove:
\[
    Pr[r\prec r'] \leq e^{\epsilon} Pr[r'\prec r]
\]
\[
    Pr[r'\prec r] \le e^{\epsilon} Pr[r\prec r']
\]
We have
\begin{align*}
Pr[r\prec r'] &= \sum_{s, s'}(kPr(\mathcal{A}(score(r)) = s)Pr(\mathcal{A}(score(r')) = s')) \\
&\leq \sum_{s, s'}(k Pr(\mathcal{A}(score(r')) = s) e^{\epsilon}Pr(\mathcal{A}(score(r)) = s')) \\
&=e^{\epsilon}\sum_{s, s'}(kPr(\mathcal{A}(score(r')) = s)Pr(\mathcal{A}(score(r)) = s')) \\
&=e^{\epsilon}Pr[r' \prec r]
\end{align*}
and
\begin{align*}
Pr[r' \prec r] &= \sum_{s, s'}(kPr(\mathcal{A}(score(r')) = s)Pr(\mathcal{A}(score(r)) = s')) \\
&\leq \sum_{s, s'}(k e^{\epsilon} Pr(\mathcal{A}(score(r)) = s)Pr(\mathcal{A}(score(r')) = s')) \\
&=e^{\epsilon}\sum_{s, s'}(kPr(\mathcal{A}(score(r)) = s)Pr(\mathcal{A}(score(r')) = s')) \\
&=e^{\epsilon}Pr[r \prec r']
\end{align*} satisfying $\epsilon$-Ordering Equality. If \[\text{Pr} [\mathcal{A}(score(r))=s] \geq \text{Pr}[\mathcal{A}(score(r'))=s]\] we still have $\epsilon$-Ordering Equality by symmetry.
\subsection{Definition 5 Proof}
Suppose we have two independent random variables $X \sim \text{Laplace}(\mu_X, b)$ and $Y \sim \text{Laplace}(\mu_Y, b)$. Suppose $\mu_X < \mu_Y$. We have
\begin{align*}
P(X < Y) &= \int_{-\infty}^{\infty} F_X(y) f_Y(y) \, dy \\
&= \int_{-\infty}^{\mu_X} F_X(y) f_Y(y) \, dy + \int_{\mu_X}^{\mu_Y} F_X(y) f_Y(y) \, dy + \int_{\mu_Y}^{\infty} F_X(y) f_Y(y) \, dy \\
&= \int_{-\infty}^{\mu_X} \frac{1}{2}\exp\left(\frac{y - \mu_X}{b}\right) \cdot \frac{1}{2b}\exp\left(\frac{y - \mu_Y}{b}\right) \, dy \\
&\phantom{={}}+ \int_{\mu_X}^{\mu_Y} \left(1 - \frac{1}{2}\exp\left(\frac{\mu_X - y}{b}\right)\right) \cdot \frac{1}{2b}\exp\left(\frac{y - \mu_Y}{b}\right) \, dy \\
&\phantom{={}}+ \int_{\mu_Y}^{\infty} \left(1 - \frac{1}{2}\exp\left(\frac{\mu_X - y}{b}\right)\right) \cdot \frac{1}{2b}\exp\left(\frac{\mu_Y - y}{b}\right) \, dy \\
&= \frac{1}{4b} \int_{-\infty}^{\mu_X} \exp\left(\frac{y - \mu_X}{b}\right) \cdot \exp\left(\frac{y - \mu_Y}{b}\right) \, dy \\
&\phantom{={}}+ \frac{1}{2b} \int_{\mu_X}^{\mu_Y} \exp\left(\frac{y - \mu_Y}{b}\right) - \frac{1}{2}\exp\left(\frac{y - \mu_Y}{b}\right)\exp\left(\frac{\mu_X - y}{b}\right) \, dy \\
&\phantom{={}}+ \frac{1}{2b} \int_{\mu_Y}^{\infty} \exp\left(\frac{\mu_Y - y}{b}\right) - \frac{1}{2}\exp\left(\frac{\mu_Y - y}{b}\right)\exp\left(\frac{\mu_X - y}{b}\right) \, dy \\
&= \frac{1}{8} \exp\left(\frac{\mu_X - \mu_Y}{b}\right) \\
&\phantom{={}}+ \frac{\mu_X - \mu_Y - 2b}{4b}\exp\left(\frac{\mu_X - \mu_Y}{b}\right) + \frac{1}{2} \\
&\phantom{={}}+ \frac{1}{2} - \frac{1}{8}\exp\left(\frac{\mu_X - \mu_Y}{b}\right)  \\
&= 1 - \frac{2b + \mu_Y - \mu_X }{4b}\exp\left(\frac{\mu_X - \mu_Y}{b}\right)
\end{align*}
Since $X, Y$ are continuous random variables, we have
\begin{align*}
P(X > Y) &= 1 - P(X < Y) \\
&= \frac{2b + \mu_Y - \mu_X}{4b}\exp\left(\frac{\mu_X - \mu_Y}{b}\right)
\end{align*}
In the context of this paper, suppose you have two commands $r, r'$ where $score(r) < score(r')$ prior to applying the Laplace noise. $X$ would be the random variable for $score(r)$ after applying the noise and $Y$ would be the random variable for $score(r')$. So, $\mu_X = score(r), \mu_Y = score(r'), b = \frac{\lambda}{\epsilon}$. $\text{Pr}[r \prec r'] = P(X < Y)$ and vice versa. 
Suppose $score(r') - score(r) = n\lambda$ for $n \geq 0$. We have
\begin{align*}
\text{Pr}[r \prec r'] &= 1 - \frac{\frac{2\lambda}{\epsilon} + n\lambda}{\frac{4\lambda}{\epsilon}}\exp\left(\frac{-n\lambda}{\frac{\lambda}{\epsilon}}\right) \\
&= 1 - \frac{2 + n\epsilon}{4}\exp\left(-n\epsilon\right) \\
\text{Pr}[r' \prec r] &= \frac{2 + n\epsilon}{4}\exp\left(-n\epsilon\right)
\end{align*} Computing the differential privacy guarantee, we have
\begin{align*}
\frac{\text{Pr}[r \prec r']}{\text{Pr}[r' \prec r]} &= \frac{1 - \frac{2 + n\epsilon}{4}\exp\left(-n\epsilon\right)}{\frac{2 + n\epsilon}{4}\exp\left(-n\epsilon\right)} \\
&= \frac{4}{2 + n\epsilon}\exp\left(n\epsilon\right) - 1 \\
&\leq \exp(n\epsilon)
\end{align*}
